# Supplementary material for: SL-CBM: Enhancing Concept Bottleneck Models with Semantic Locality for Better Interpretability
Source: arXiv:2601.12804 source file (2026-01-19)
Supplement: Supplementary file 1 [file supp.tex]

\clearpage

\title{Supplementary material for \\
``SL-CBM: Enhancing Concept Bottleneck Models with Semantic Locality for Better Interpretability''}

% % COMMENT OUT \maketitle FROM main.tex FOR \maketitle TO WORK HERE
\maketitle

% PAGE NUMBER SET TO 1
\setcounter{page}{1}

% START APPENDIX
\appendix

% NUMBERING

%------------------------------------------------------------------------------

\section*{Introduction}
In the supplementary material, we first present ablation results conducted on a small dataset, demonstrating that hyperparameter tuning performed on limited data can generalize effectively to larger datasets. These experiments highlight the practical adaptability of our method across different data scales. In addition, we provide extended experimental results of our attack method applied to other datasets, further validating its robustness and generalizability.

\section{Ablation Studies on a Small-Scale Dataset}

We extend our experiments on the RIVAL-10 dataset as discussed in the Ablation section of the main paper. Specifically, we conduct an ablation study on the loss function parameters $\lambda_e$ (for Entropy Loss) and $\lambda_c$ (for Contrastive Loss), while fixing $\lambda_{ce} = 1$ for the Cross-Entropy Loss and $\lambda_{ca} = 10^4$ for the Concept Accuracy Loss.

The value of $\lambda_e$ is varied over the set ${0, 0.1, 0.5, 1.0, 1.5, 2.0, 5.0, 10.0}$, and $\lambda_c$ is set to either $1$ or $0$ to assess its contribution. Additionally, beyond using the full test set for hyperparameter tuning, we explore two alternative data conditions: using half of the dataset (\ie, 50\%) and a fifth of the dataset (\ie, 10\%). 

The experimental results are presented in Figure~\ref{fig:ablation-E-small}. In the visualization, we use distinct markers to indicate whether the Contrastive Loss ($\lambda_c$) is applied, and different colors to represent the scale of data used in each experiment.

Overall, the results show consistent performance trends across different data scales. Although there is one outlier observed when using the full dataset in the IoU and Dice metrics, the selected hyperparameters remain optimal when considering the trade-offs across all eight evaluation metrics.

These findings suggest that effective hyperparameter selection can be performed on smaller subsets of data, with the resulting configuration generalizing well to larger datasets. This highlights the practical adaptability and efficiency of SL-CBM in real-world scenarios.

\input{tex/table/ablation-E-small}

\begin{table*}[thbp]
    \centering
    \setlength{\tabcolsep}{8pt}
    \begin{tabular}{lr|cc|cc|cc|cc|cc} \toprule
     \multicolumn{2}{c|}{\mr{4}{Method}} & \multicolumn{4}{c|}{\mr{3}{Accuracy}} & \mc{6}{Locality Faithfulness (Without Annotation)} \\\cmidrule{7-12}
     &&\multicolumn{4}{c|}{} &\multicolumn{2}{c|}{AD $\downarrow$}&\multicolumn{2}{c|}{AI $\uparrow$}&\multicolumn{2}{c}{AG $\uparrow$}\\ \cmidrule{3-12}
     && Concept&Class & NEC-5& ANEC &$S_{\cC_{gt}}$&$S_{l_{gt}}$&$S_{\cC_{gt}}$&$S_{l_{gt}}$&$S_{\cC_{gt}}$&$S_{l_{gt}}$\\\midrule
         \mr{2}{PCBM}&ResNet50 & 47.52 & 72.46 & 72.46 & 72.46 & 1.06 & 1.15 & 29.86 & 25.54 & 0.36 & 0.28 \\
         &ViT-B16 &  42.36 & 67.53 & 60.71 & 64.12 & \textbf{0.37} & \textbf{0.37} & \textbf{83.34} & \textbf{82.68} & \textbf{25.63} & \textbf{22.96}\\\midrule
        \multicolumn{2}{c|}{CSS} & 71.54 & \textbf{91.27} & \textbf{91.21} & \textbf{91.24} & 24.16 & 26.42 & 45.63 & 41.46 & 21.80 & 19.88\\ \midrule
         \rowcolor{cyan!10}
          \multicolumn{2}{c|}{SL-CBM}& \textbf{77.37} & 85.99 & 85.82 & 85.91 & 23.11 & 21.32 & 42.21 & 42.19 & 17.14 & 14.69\\
         \bottomrule
    \end{tabular}
    \caption{Comparison of SL-CBM with state-of-the-art CBMs on CelebA in terms of accuracy, as well as locality faithfulness metrics with annotation (IoU, Dice, C-IoU) and without annotation (AD, AI, AG) at both concept-level and class-level. $\uparrow$ signifies that a higher value is preferable for the metric, while $\downarrow$ indicates that a lower value is better. All values are presented as percentages. The best results are highlighted in bold.}
    \label{tab:cp-celeba}
\end{table*}

\section{Additional Experimental Results}

\paragraph{Comparison on CelebA.}

We evaluate performance on the CelebA dataset~\cite{liu2015faceattributes}, following the experimental setup proposed by \citet{kalampalikis2025towards}. In this setting, evaluation is limited to the binary classification task of detecting the \emph{smiling} attribute, using a concept set composed of only seven facial attributes: \emph{Bags Under Eyes}, \emph{High Cheekbones}, \emph{Mouth Slightly Open}, \emph{Rosy Cheeks}, \emph{Double Chin}, \emph{Arched Eyebrows}, \emph{and Narrow Eyes}. This constitutes an extreme scenario, characterized by a highly constrained concept space and a binary classification task (smiling vs. not smiling), which may limit the expressive power and discriminative capacity of concept-based models.

\input{tex/table/celebA_intervention}

To ensure consistency across datasets, we do not perform hyperparameter tuning specifically for CelebA, but instead adopt the same settings used for RIVAL-10. The results, presented in Table~\ref{tab:cp-celeba}, indicate that CSS achieves the highest performance in both class accuracy and interpretable confidence, while PCBM, in contrast, performs better on locality faithfulness. SL-CBM shows superior concept accuracy but is generally outperformed by CSS in other metrics.
We do not interpret these results as a failure of our method. Rather, they highlight a limitation arising from the experimental constraints. Specifically, when both the number of classes and the size of the concept set are extremely limited, the ability of concept-based models to fully leverage their interpretability and generalization strengths may be reduced.

\input{tex/table/rival10_intevention}

\paragraph{More Experiments for Intervention.}
We conduct the intervention experiments from the main paper on datasets with relatively small concept sets, \ie, CelebA and RIVAL-10. The corresponding results are presented in Figure~\ref{fig:intervention-celeba} and Figure~\ref{fig:intervention-rival10}. These experiments reveal that replacing predicted concepts with ground-truth concepts leads to a decrease in overall performance across all methods. This counterintuitive phenomenon has also been observed in prior work, and is commonly attributed to the limited size of the concept set, which may cause the models to overfit to the training data.

Notably, the intervention curves for CelebA exhibit more noise and a sharper performance drop compared to RIVAL-10. This discrepancy can be explained by the smaller concept set used in CelebA, which further restricts the model’s capacity to generalize under intervention. These findings underscore the importance of having a sufficiently large and diverse concept set for CBMs to be effective and robust.

Nevertheless, we emphasize that even in this challenging setting, SL-CBM demonstrates the most stable behavior, exhibiting the smallest performance degradation under intervention among all evaluated CBMs. This suggests that SL-CBM has learned more faithful concept-based features, even when the concept space is severely constrained.

{
    \small
    \bibliography{reference}
}
